# Supplementary material for: Accounting for Input Noise in Gaussian Process Parameter Retrieval
Source: arXiv:2005.09907 source file (2020-05-20)
Supplement: Supplementary file 1 [file exp_params.tex]

This graphs in sub-figure \ref{fig:param} demonstrate how the Spearman correlation coefficient in particular changes as the number of samples and the number training samples change. Regardless of the configuration we tried, we consistently obtained a higher Spearman correlation coefficient with the eGP standard deviation. 

\begin{figure}[h!]
\begin{center}
% 		\begin{tabular}{c}
% 			\includegraphics[height=3cm,width=4cm]{toy_example_1d/fit/data.png}
% 		\end{tabular}
% \setlength{\tabcolsep}{2pt}
\begin{tabular}{cc}
%$\dfrac{\partial g(\x^*)}{\partial f(\x^*)}$ &
\includegraphics[height=3cm,width=4cm]{images/experiment/mae/full_orbit/spearman/20131001_krr_mae_spear_mae_10.png} &
\includegraphics[height=3cm,width=4cm]{images/experiment/r2/full_orbit/20131001_krr_r2_10.png}
\\
(a) 10  dimensions
\\
\includegraphics[height=2.75cm,width=3.75cm]{images/experiment/mae/full_orbit/spearman/20131001_krr_mae_spear_mae_25.png}  &
\includegraphics[height=2.75cm,width=3.75cm]{images/experiment/r2/full_orbit/20131001_krr_r2_25.png}
\\
(b) 25  dimensions
\\
\\
\includegraphics[height=3cm,width=4cm]{images/experiment/mae/full_orbit/spearman/20131001_krr_mae_spear_mae_50.png}  &
\includegraphics[height=3cm,width=4cm]{images/experiment/r2/full_orbit/20131001_krr_r2_50.png}
\\
(c) 50  dimensions

\end{tabular}
\vspace{-0.0cm}
\caption{This figure shows the experimental results to measure the Pearson correlation coefficient between the variance and the mean squared error (MSE). The left column showcased the mean Spearman correlation coefficient and associated standard deviation for a different number of training samples under a different number of dimensions (a) - (c). The right column showcases the mean  for the model fit (R2 score) and the mean for the residual errors (Root Mean Squared) for different numbers of training samples under different numbers of dimensions (a) - (c). All values have an associated error bar as a result of the 10 trials where the training data was randomly sampled.} 
\label{fig:param}
\end{center}
\end{figure}
