# Supplementary material for: Accounting for Input Noise in Gaussian Process Parameter Retrieval
Source: arXiv:2005.09907 source file (2020-05-20)
Supplement: Supplementary file 2 [file correlation.tex]

\subsection{Correlation}

The plots in figure \ref{fig:corr} display a clear difference in the distribution of the points along the standard deviation axis. The correlation coefficients also support the notion that the standard deviation of the eGP is more correlated to the absolute error. This corresponds to sub-figure (\ref{fig:error}c) having a more pronounced color scheme between the lowest and highest standard deviation.

\begin{figure}[t!]
\begin{center}

\begin{tabular}{cc}
%$\dfrac{\partial g(\x^*)}{\partial f(\x^*)}$ &
\hspace{-5mm}
\includegraphics[height=4cm,width=5cm]{images/experiment/correlation/mae/full_standard_corr_mae_mean.png} &
\hspace{-8mm}
\includegraphics[height=4cm,width=5cm]{images/experiment/correlation/mae/full_variance_corr_mae_mean.png}
% \vspace{-10mm}
\\
% \vspace{-10mm}
(a) GP &
(b) eGP
% \vspace{5mm}

\end{tabular}

\caption{This figure shows the Standard Deviation versus the Absolute Error for the (a) standard GP and (b) the GP with the enhanced variance estimate.} 
\label{fig:corr}
\end{center}
\end{figure}
