# Supplementary material for: Accounting for Input Noise in Gaussian Process Parameter Retrieval
Source: arXiv:2005.09907 source file (2020-05-20)
Supplement: Supplementary file 3 [file literaturereview.tex]

In the literature, an early look at dealing with uncertain inputs is known as errors-in-variables regression \cite{Dellaportas1995}. In relation to GPs, the early approaches to dealing with input uncertainty came from \cite{Girard2003}. They use local approximations of the test points from the posterior of GP function by using the Taylor approximation of the predictive mean and variance functions. Observations from \cite{Solak2003} note that derivatives of GPs are GPs as well so the derivatives have a closed-form mean and variance function. However, their approach resulted in a minimum of 2nd order derivatives of the covariance function and 3rd order to calculate the gradients for minimizing the maximum likelihood. This is computational intractable when the number of points and dimensions increases. Another problem with this approach is that integrating over all possible trial points may not result in a Gaussian distribution. One can force the resulting distribution to be Gaussian by using the approximate moments approach. This was started by \cite{Girard2003a, Quinonero-Candela2003} and further developed in \cite{Deisenroth2009, Deisenroth2011}. The Taylor approximation and moment matching approaches only look at the uncertainty in the test points. They assume some noise in the $x$ inputs but only take them into account during the predictions. \cite{Dallaire2011} applies an uncertainty incorporating covariance function and similarly in \cite{Girard2003}.  But this case is only applicable if the error in the inputs are explicitly known and does not make adjustments to the model from the posterior information.

One can imagine that in regions where there is a high gradient where the output value is rapidly changing, the input measurements corrupted by noise will be more important in these regions as opposed to regions where the output is almost constant. Figure \ref{fig:derivative} illustrates this affect as when there is a gradient, the noisy inputs affect the output of the function more than in regions where the output is almost constant. The Noise-Input Gaussian Process (NIGP) method \cite{Mchutchon2011} takes into account the posterior data with the same argument about using a combination of the gradient and the input error covariance matrix. This method processes the input noise through the Taylor expansion as being proportional to the derivative of the predictive function. Optionally, one could add an additional order which would account for the uncertainty in the gradient itself however they note that this additional error is almost neglegible in their experiments. These noise parameters for the inputs are fitted which can give an input noise variance estimate per dimension. The downside to this method is that it does not scale well because one has to iteratively fit multiple GPs and thus it cannot be applied to large datasets. We will elaborate more on this method in the upcoming section as it is the basis of our experiments. \cite{Bijl2016} improves upon this method further by introducing a fully independent training conditional (FITC) augmentation to train the GP online. This method scales and is a great addition to the NIGP framework.

\begin{figure}
\begin{center}
% 		\begin{tabular}{c}
% 			\includegraphics[height=3cm,width=4cm]{toy_example_1d/fit/data.png}
% 		\end{tabular}
% \setlength{\tabcolsep}{2pt}
\begin{tabular}{ccc}
%$\dfrac{\partial g(\x^*)}{\partial f(\x^*)}$ &
\hspace{-7mm}
\includegraphics[height=35mm,width=35mm]{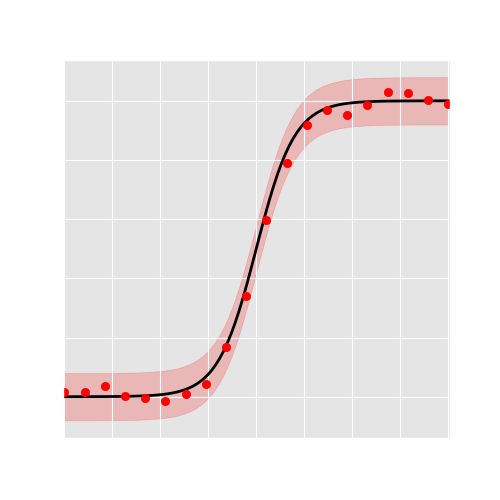} &
\hspace{-10mm}
\includegraphics[height=35mm,width=35mm]{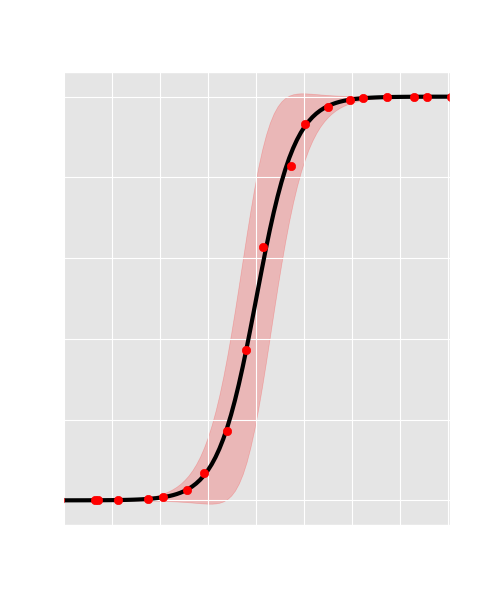} &
\hspace{-10mm}
\includegraphics[height=35mm,width=35mm]{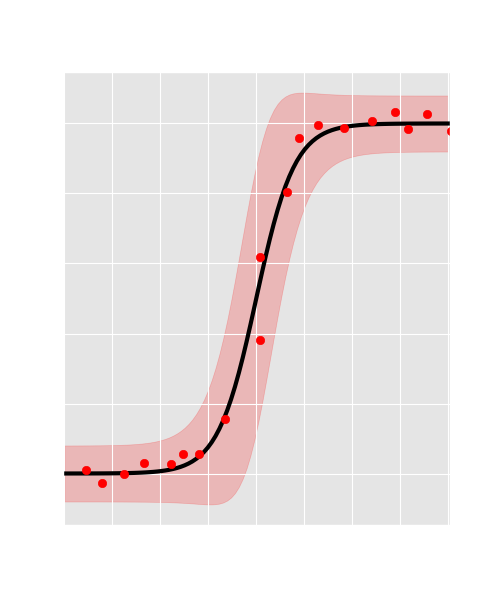}
\\
\hspace{-5mm}(a) & \hspace{-5mm}(b) & \hspace{-5mm}(c)

\end{tabular}
% \vspace{-0.25cm}

\caption{This is an illustration showing the effects of (a) only noise for the outputs $\y$, (b) only noise for the inputs $\x$ and (c) noise for both the inputs $\x$ and the outputs $\y$.} \label{fig:derivative}
\end{center}
\end{figure}

There are methods that are not in the same family as the Taylor approximation and moment-matching methods but still seek to characterize the input noise better. One family of approaches uses heteroscedastic noise models \cite{Kersting2007}, as they model the noise directly in the training and testing phase. In this approach, a function is applied to the noise coefficient $\sigma_y^2$. However, it is an approximation and does not exploit the structure of the input noise specifically yet adds more degrees of freedom to the learning algorithm. 

\textbf{(TODO: part about inverse uncertainty (Baumgaertel et al., 2014))}

The variational approach \cite{Titsias2010} chooses a variational distribution that approximates the maximum likelihood of the GP model under the assumption of uncertainty in the inputs. Utilizing the GP Latent Variable Model (GPLVM) \cite{Lawrence2003}, they show how this can be exploited to approximate the distribution of the input space. Furthermore, due to the emergence of deep learning architectures and improved methodologies of minimizing the variational loss function \cite{Damianou2016}, this method has been shown to scale very well. In addition, the emergence of multi-layer deep GP networks allows one to measure the uncertainty in the inputs through each layer \cite{Damianou2013}. Interestingly, it has the same idea as a dynamical system which motivated many of the input-noise estimate methods above. In the dynamical setting, once again, it assumes that output $t$ is function of $t-1$ where it is obvious that there is noise in this estimate. Similarly, a deep GP chains single GPs together through the layers and propagates the result of each GP through each subsequent layer. Using the variational inference methods assuming latent variables for each input, this also naturally accounts for the noise in the inputs.

We conclude this section by introducing our contribution in this letter. We take the original formulation of the NIGP and augment it so that it matches our application. Some key ideas to consider is that we provide a formulation that is simplier and less expensive yet still captures the input error and its relation to the derivative of the function. The following section gives the formulation from the NIGP perspective and concludes with our final formulation.
